# Supplementary material for: Post-shock-revival evolutions in the neutrino-heating mechanism of core-collapse supernovae
Source: arXiv:1209.4824 source file (2013-05-02)
Supplement: Supplementary file 1 [file appendix.tex]

\begin{appendix}

In this appendix, we represent our treatment of neutrino interactions, 
such as neutrino opacity, optical depth, and emission rates, 
which are chiefly followed by \citet{ruffert96}.

\section{Neutrino opacity}

\subsection{degeneracy parameters of neutrinos}

We assume that the neutrino spectra are represented by Fermi-Dirac distributions
for the temperature $T$, which is taken to be that of the gas temperature, 
and chemical potential $\mu_{\nu_i}$. 
Hereafter, we set the Boltzmann constant $k_{\rm B}$ to be unity. 
The neutrino degeracy parameter $\eta_{\nu_i} = \mu_{\nu_i}/T$ is set to be 
\begin{eqnarray}
 \eta_{\nu_x} &=& 0, \\
 \eta_{\nue} &=& \eta^{\rm ceq}_{\nue} ( 1 - \exp(-\tau_{\nue})), \\
 \eta_{\nube} &=& \eta^{\rm ceq}_{\nube} ( 1 - \exp(-\tau_{\nube})),
\end{eqnarray}
for heavy-lepton, electron, and anti-electron neutrinos, respectively.
Here $\eta^{\rm ceq}_{\nue}$ is the degeneracy parameter for $\nue$
at chemical equilibrium with the stellar matter,
\begin{equation}
 \eta^{\rm ceq}_{\nue} = - \eta^{\rm ceq}_{\nube} = 
  \eta_e +\eta_p -\eta_n -Q/T
\end{equation}
where 
$\eta_e$ is the degeneracy parameters of electrons (including electron rest mass),
$\eta_p$ and $\eta_n$ are the degeneracy parameters of protons and neutrons, 
respectively (without rest masses), and
$Q = 1.2935 \mev$ is the rest-mass-energy difference between a neutron ans a proton.
The optical depths of neutrino interactions $\tau_{\nu_i}$ 
are presented in the following section.
We note that $\eta_{\nue}$ and $\eta_{\nube}$ in the limit of transparent matter
are set to vanish, as in \citet{ruffert96}.

\subsection{opacities for neutrino scattering}

We represent spectrally averaged opacities for scattering of neutrinos $\nu_i$
by nuclei $N_i$ (neutrons, protons, or heavy nuclei)|\citep{ruffert96, tubbs75} as 
\begin{equation}
 \kappa_{s,j}(\nu_i,N_i) = C_{s,N_i} \sigma_0
 \left(\frac{\rho \, Y_{N_i}}{M_{\rm amu}}\right)
 \left(\frac{T}{m_e c^2}\right) \frac{F_{4+j}(\eta_{\nu_i})}{F_{2+j}(\eta_{\nu_i})},
\end{equation}
where $m_e$ is the llectron rest mass, $c$ the speed of light, 
$M_{\rm amu}$ the atomic mass units, 
$\sigma_0 = 1.76 \times 10^{-44} \rm \cm^2$, 
and $Y_{N_i}$ number fractions.
For $j=0$ and $j=1$
one obtains the opacities for neutrino-number and -energy transport, respectively.
Here $C_{s,n} = (1+5\alpha^2)/24$ and $C_{s,p} = [4(C_V -1)^2 +5\alpha^2]/24$
with $C_v = 0.5 + 2 \sin^2 \theta_W$, $\theta_W \simeq 0.23$, and 
$\alpha \simeq 1.25$, and
$C_{s,N} = [A - 2(2-C_V -C_A) Z]^2/16$ for heavy nuclei with mass number $A$
and atomic number $Z$ using $C_A = 1/2$.
$F_n$ is a Fermi integral given by
\begin{equation} 
    F_n(z)= \int_0^\infty \frac{x^n dx}{e^{x-z}+1} \label{fermi_int}
\end{equation}
and can be efficiently evaluated via series expansions~\citep{takahashi78}. 
%% ref %% Takahashi, 1978

\subsection{opacities for neutrino absorptions}

We represent spectrally averaged opacities for neutrino absorption on
neclei $N_i$ (neutrons or protons)~\citep{ruffert96, tubbs75} as 
\begin{eqnarray}
 \kappa_{a,j}(\nue,n) &=& \frac{1 +3 \alpha^2}{4}\sigma_0
 \left(\frac{\rho \, Y_{n}}{M_{\rm amu}}\right)
 \left(\frac{T}{m_e c^2}\right) \frac{F_{4+j}(\eta_{\nue})}{F_{2+j}(\eta_{\nue})}
 P_{e^-}, \\
 \kappa_{a,j}(\nube,p) &=& \frac{1 +3 \alpha^2}{4}\sigma_0
 \left(\frac{\rho \, Y_{p}}{M_{\rm amu}}\right)
 \left(\frac{T}{m_e c^2}\right) \frac{F_{4+j}(\eta_{\nube})}{F_{2+j}(\eta_{\nube})}
 P_{e^+}
\end{eqnarray}
where $P_{e^-}$ and $P_{e^+}$ are the phase space blocking of the electrons
and positrons, respectively, and we adopt the approximate expresions,
\begin{eqnarray}
P_{e^-} &\simeq& \left\{ 1 + 
 \exp \left[-\left( \frac{F_5(\eta_{\nue})}{F_4(\eta_{\nue})} -\eta_e\right)
\right]\right\}^{-1} \\
P_{e^+} &\simeq& \left\{ 1 + 
 \exp \left[-\left( \frac{F_5(\eta_{\nube})}{F_4(\eta_{\nube})} +\eta_e\right)
\right]\right\}^{-1} \\
\end{eqnarray}

\subsection{total opacities}

Total opacities are estimated for $\nue$, 
\begin{equation}
 \kappa_{t,j}(\nue) = \kappa_{s,j}(\nue,n) +\kappa_{s,j}(\nue,p)
+\kappa_{s,j}(\nue,N_{A,Z}) +\kappa_{a,j}(\nue,n),
\end{equation}
for $\nube$, 
\begin{equation}
 \kappa_{t,j}(\nube) = \kappa_{s,j}(\nube,n) +\kappa_{s,j}(\nube,p)
+\kappa_{s,j}(\nube,N_{A,Z}) +\kappa_{a,j}(\nube,p),
\end{equation}
and for $\nux$, 
\begin{equation}
 \kappa_{t,j}(\nux) = \kappa_{s,j}(\nux,n) +\kappa_{s,j}(\nux,p)
+\kappa_{s,j}(\nux,N_{A,Z}),
\end{equation}
where $N_{A,Z}$ is a heavy nuclei with mass number $A$ and atomic number $Z$.

\section{neutrino emission rates through transperent material}

\subsection{capture processes}

The emission rates of $\nue$ per unit volume and unit time 
via electron capture on protons is given by
\begin{equation}
 R_{\rm cap} (\nue) = \frac{1+3 \alpha^2}{8} 
 \frac{8\pi}{(h c)^3}
 \frac{\sigma_0 c}{(m_e c^2)^2} 
 \left(\frac{\rho \, Y_{p}}{M_{\rm amu}}\right)
 T^5 F_{4}(\eta_e)  P_{{\rm cap},\nue},
\end{equation}
and those of $\nube$ via positron capture on neutrons by
\begin{equation}
 R_{\rm cap} (\nube) = \frac{1+3 \alpha^2}{8} 
 \frac{8\pi}{(h c)^3}
 \frac{\sigma_0 c}{(m_e c^2)^2} 
 \left(\frac{\rho \, Y_{n}}{M_{\rm amu}}\right)
 T^5 F_{4}(-\eta_e)  P_{{\rm cap},\nube},
\end{equation}
where $h$ is the Planck constant, and 
$P_{{\rm cap},\nue}$ and $P_{{\rm cap},\nube}$ are 
the phase space blocking of $\nue$ and $\nube$ for capture processes, respectively, 
and are approximately taken into account by
\begin{eqnarray}
P_{{\rm cap},\nue} &\simeq& \left\{ 1 + 
 \exp \left[-\left( \frac{F_5(\eta_{e})}{F_4(\eta_e)} -\eta_{\nue}\right)
\right]\right\}^{-1} \\
P_{{\rm cap},\nube} &\simeq& \left\{ 1 + 
 \exp \left[-\left( \frac{F_5(-\eta_{e})}{F_4(-\eta_e)} -\eta_{\nube}\right)
\right]\right\}^{-1} \\
\end{eqnarray}

The energy emission rates of $\nue$ per unit volume and unit time 
via electron capture on protons is given by
\begin{equation}
 Q_{\rm cap} (\nue) = \frac{1+3 \alpha^2}{8} 
 \frac{8\pi}{(h c)^3}
 \frac{\sigma_0 c}{(m_e c^2)^2} 
 \left(\frac{\rho \, Y_{p}}{M_{\rm amu}}\right)
 T^6 F_{5}(\eta_e)  P_{{\rm cap},\nue},
\end{equation}
and those of $\nube$ via positron capture on neutrons by
\begin{equation}
 Q_{\rm cap} (\nube) = \frac{1+3 \alpha^2}{8} 
 \frac{8\pi}{(h c)^3}
 \frac{\sigma_0 c}{(m_e c^2)^2} 
 \left(\frac{\rho \, Y_{n}}{M_{\rm amu}}\right)
 T^6 F_{5}(-\eta_e)  P_{{\rm cap},\nube},
\end{equation}

\subsection{pair processes}

The emission rates of $\nue$ per unit volume and unit time 
via electron-positron pair annihilations is given by
\begin{equation}
 R_{\rm pair} (\nue) = R_{\rm pair} (\nube) = 
\frac{C_V^2+ C_A^2}{18} 
 \left(\frac{8\pi}{(h c)^3}\right)^2
 \frac{\sigma_0 c}{(m_e c^2)^2} 
 T^8 F_{3}(\eta_e) F_{3}(-\eta_e) 
 P_{{\rm pair},\nue} P_{{\rm pair},\nube},
\end{equation}
where 
$P_{{\rm pair},\nue}$ and $P_{{\rm pair},\nube}$ are 
factors for the phase space blocking of $\nue$ and $\nube$ for pair processes, 
respectively.
The factor for $\nu_i$ is approximately expressed as
\begin{equation}
P_{{\rm pair},\nu_i} \simeq \left\{ 1 + 
 \exp \left[-\left( 
\frac{1}{2}\frac{F_4(\eta_{e})}{F_3(\eta_e)} 
+\frac{1}{2}\frac{F_4(-\eta_{e})}{F_3(-\eta_e)} 
 -\eta_{\nu_i}\right)
\right]\right\}^{-1}.
\end{equation}

The emission rates of $\nux$ via pair annihilations is given by
\begin{equation}
 R_{\rm pair} (\nux) = 
 \frac{(C_V -C_A)^2 +(C_V +C_A -2)^2}{9} 
 \left(\frac{8\pi}{(h c)^3}\right)^2
 \frac{\sigma_0 c}{(m_e c^2)^2} 
 T^8 F_{3}(\eta_e) F_{3}(-\eta_e) 
 (P_{{\rm pair},\nux})^2.
\end{equation}

The energy emission rates of $\nue$ and $\nube$ per unit volume and unit time 
via electron-positron pair annihilations are given by
\begin{equation}
 Q_{\rm pair} (\nue) = Q_{\rm pair} (\nube) = 
\frac{C_V^2+ C_A^2}{36} 
 \left(\frac{8\pi}{(h c)^3}\right)^2
 \frac{\sigma_0 c}{(m_e c^2)^2} 
 T^9 [ F_{4}(\eta_e) F_{3}(-\eta_e) + F_{3}(\eta_e) F_{4}(-\eta_e) ]
 P_{{\rm pair},\nue} P_{{\rm pair},\nube},
\end{equation}
and the rates for $\nux$ are given by
\begin{equation}
 Q_{\rm pair} (\nux) = 
 \frac{(C_V -C_A)^2 +(C_V +C_A -2)^2}{18} 
 \left(\frac{8\pi}{(h c)^3}\right)^2
 \frac{\sigma_0 c}{(m_e c^2)^2} 
 T^9 [ F_{4}(\eta_e) F_{3}(-\eta_e) + F_{3}(\eta_e) F_{4}(-\eta_e) ]
 (P_{{\rm pair},\nux})^2.
\end{equation}

\subsection{plasmon decay processes}

The emission rates of $\nue$ and $\nube$ per unit volume and unit time
via plasmon decay are given by
\begin{equation}
 R_{\rm plas} (\nue) = R_{\rm plas} (\nube) = 
C_V^2 \frac{\pi^3}{3 \alpha_* (hc)^6} 
 \frac{\sigma_0 c}{(m_e c^2)^2} 
 T^8 \gamma^6 e^{-\gamma}(1+\gamma)
 P_{{\rm plas},\nue} P_{{\rm plas},\nube},
\end{equation}
where $\alpha_* = 1/137.036$ is the fine-structure constant, 
$\gamma = \gamma_0 \sqrt{\eta_e^2 +\pi~2/3}$ with 
$\gamma_0 = 2\sqrt{\alpha_*/3\pi} = 5.565 \times 10^{-2}$, 
$P_{{\rm plas},\nue}$ and $P_{{\rm plas},\nube}$ are 
factors for the phase space blocking of $\nue$ and $\nube$ for 
plasmon decay processes, respectively.
The factor for $\nu_i$ is approximately expressed as
\begin{equation}
P_{{\rm plas},\nu_i} \simeq \left\{ 1 + 
 \exp \left[-\left( 1+
\frac{1}{2}\frac{\gamma^2}{1+\gamma} -\eta_{\nu_i}\right)
\right]\right\}^{-1}.
\end{equation}

The emission rates of $\nux$ via plasmon decay is given by
\begin{equation}
 R_{\rm plas} (\nux) = 
(C_V-1)^2 \frac{4\pi^3}{3 \alpha_* (hc)^6} 
 \frac{\sigma_0 c}{(m_e c^2)^2} 
 T^8 \gamma^6 e^{-\gamma}(1+\gamma)
 (P_{{\rm plas},\nux})^2
\end{equation}

The energy emission rates of $\nu_i$ per unit volume and unit time 
via plasmon decaye is given by
\begin{equation}
 Q_{\rm plas} (\nu_i) =  R_{\rm plas} (\nu_i) \cdot
T \left( 1 + \frac{1}{2}\frac{\gamma^2}{1+\gamma} \right)
\end{equation}

\section{neutrino leakage treatment}

The optical depth for transport of neutrinos $\nu_i$ is 
\begin{equation}
 \tau_{\nu_i,j}(r) = \int^\infty_r \kappa_{t,j} (\nu_i) \, dr,
\end{equation}
where for $j=0$ and $j=1$
one obtains the depths for neutrino-number and -energy transport, respectively.

\newpage

\section{Neutrino treatment}
The rates that we use in the simulations are smooth interpolations
between diffusion and local production rates.
If we denote for a given neutrino species  $\nu_i$ the number
emission rates by $R_{\nu_i}$ per volume and energy emission rates per volume 
by $Q_{\nu_i}$, our prescription for the  {\em effective} rates reads
    
\begin{eqnarray} 
	R_{\nu_i}^{ef} = 
                        R_{\nu_i}^{loc} \left(1+
                        \frac{R_{\nu_i}^{loc}}{R_{\nu_i}^{dif}} \right)^{-1}
                        \label{Ref}\\
	Q_{\nu_i}^{ef} = 
                        Q_{\nu_i}^{loc} \left(1+
	                \frac{Q_{\nu_i}^{loc}}{Q_{\nu_i}^{dif}}\right)^{-1}.
                        \label{Qef}
\end{eqnarray}
This ansatz is similar to the one used in Ruffert et al. (1996).
%\cite{ruffert97a}.
Here the quantities with the superscript ``$loc$'' denote the locally produced 
rates of number and energy while the superscript ``$dif$'' refers to the
diffusion rates that are further specified below. 
In the transparent regime, where the diffusion time scale $T^{dif}_{\nu_{i}}$
is short, and therefore $R_{\nu_i}^{dif} \gg R_{\nu_i}^{loc}$ and 
$Q_{\nu_i}^{dif} \gg Q_{\nu_i}^{loc}$ 
all the locally produced neutrinos stream out freely. In the very opaque 
regime, where $T^{dif}_{\nu_{i}}$ is large, the neutrinos leak out on the 
diffusion time scale. Therefore both limits are treated correctly, the 
regime inbetween these limits is handled via interpolation.\\
The mean neutrino energy of each SPH-particle (particle index suppressed) 
is then found from
\begin{equation}
	E^{ef}_{\nu_i}= \frac{\sum_r Q^{ef}_{\nu_i,r}}{\sum_r 
	                 R^{ef}_{\nu_i,r}}, \label{Eeff}
\end{equation}
where $r$ labels all reactions producing neutrinos of type ${\nu_i}$.
Note, that these (mean) energies are used exclusively for book-keeping 
purposes, in all places where a dependence on neutrino energies occurs, we 
integrate cross-sections over a Fermi-distribution (see below).\\
To characterize the average neutrino energies of the total system we use 
rms energies given by
\begin{equation}
\epsilon_{\nu_i}= \sqrt{ \frac{\sum_j \tilde{R}^{ef}_{\nu_i,j} 
(E^{ef}_{\nu_i,j})^2}{\sum_j \tilde{R}^{ef}_{\nu_i,j}}},
\label{mean_E}
\end{equation}
where $j$ labels the SPH-particles and $\tilde{R}^{ef}_{\nu_i,j}$ is the rate
of neutrino number emission of particle $j$ (not to be confused with the rate
{\em per volume}, $R^{ef}_{\nu_i,j}$).\\
We have tested this scheme in spherical symmetry against
stationary state Boltzmann transport (Mezzacappa \& Messer 1999). 
To this end we determined the neutrino properties
for a frozen matter background. The background properties ($\rho,T$ and $Y_e$)
were either taken from neutron star merger (Rosswog \& Davies 2002) or core 
collapse supernova simulations (Liebend\"orfer et al. 2002). 
While the rms neutrino energies agree within 20 $\%$ the 
accuracy of the luminosities depends on the importance of the semi-transparent
regime where the interpolation (eqs. (\ref{Ref}) and (\ref{Qef})) is applied. 
In the worst case we found that our scheme overestimates the luminosities
by a factor 3-4.

\subsection{Free Emission Rates}\label{app_em_rate}
In the following we will neglect the electron mass and the nucleon mass 
difference, $Q= m_n - m_p = 1.2935$ MeV, in all the cross sections 
%\cite{tubbs75}
(Tubbs \& Schramm 1975). This is 
appropriate for our purposes and largely simplifies the involved rate 
expressions. 
We further assume the neutrino temperature to be identical to the local matter
temperature and, where necessary, we assume the neutrinos to follow a 
Fermi-distribution. The chemical potentials of the $\nu_x$ are generally
assumed to vanish, for $\nu_e$ and $\bar{\nu}_e$ we apply the equilibrium 
values
\begin{equation}
    \mu_{\nu_e}= - \mu_{\bar{\nu}_e} = \bar{\mu}_e - \hat{\mu} - Q,
	\label{beta_eq}
\end{equation}
wherever they occur in the sequel. Here $\bar{\mu}_e$ is the electron chemical 
potential (with rest mass) and $\hat{\mu}$ is the difference in the neutron 
and proton chemical potentials (without rest mass). 
Degeneracy parameters $\mu_i/T$ are denoted by $\eta_i$, temperatures are 
always in units of energies.\\
With these approximations and ignoring momentum transfer to the 
nucleon (Bruenn 1985) 
%\cite{bruenn85}
 the {\em electron capture} rate per volume reads 
\begin{equation} 
    R_{EC}= \beta \; \eta_{pn} T^5 F_4(\eta_e),\label{REC},
\end{equation}
with 
\begin{equation}
 \beta= \frac{\pi}{h^3 c^2} \frac{1+3 \alpha^2}{(m_e c^2)^2} 
    \sigma_0.
\end{equation}
Here $h$ is Planck's constant and $c$ the speed of light, $\alpha 
\approx 1.25$, $m_e$ is the electron mass, $\sigma_0\approx 1.76\cdot 10^{-44}$cm$^2$. $F_n$ is a Fermi integral given by
\begin{equation} 
    F_n(z)= \int_0^\infty \frac{x^n dx}{e^{x-z}+1} \label{fermi_int}
\end{equation}
and can be efficiently evaluated via series expansions 
%\cite{takahashi78}. 
(Takahashi et al. 1978).
The factor $\eta_{pn}$ given by
\begin{equation} 
    \eta_{pn}= \frac{n_n-n_p}{exp(\hat{\mu}/T)-1}, 
\end{equation}
 takes into account the nucleon final state blocking and
reduces in the non-degenerate limit to the proton number density $n_p$, 
$n_n$ refers to the neutron number density.
Following the analogous procedure one finds for the energy emission rate
\begin{equation} 
    Q_{EC}= \beta \, \eta_{pn} T^6 F_5(\eta_e),
\end{equation}
and for the mean energy of the emitted neutrinos
\begin{equation} 
    \langle E_{\nu_e} \rangle_{EC}= \frac{Q_{EC}}{R_{EC}} = 
    T \frac{F_5(\eta_e)}{F_4(\eta_e)}.
\end{equation}	
The corresponding rates for {\em positron captures} read
\begin{equation} 
    R_{PC}= \beta \, \eta_{np} T^5 F_4(-\eta_e),
\end{equation}
\begin{equation} 
    Q_{PC}= \beta \, \eta_{np} T^6 F_5(-\eta_e),
\end{equation}
\begin{equation} 
    \langle E_{\bar{\nu}_e} \rangle_{PC}= 
    T \frac{F_5(-\eta_e)}{F_4(-\eta_e)},
\end{equation}
where $\eta_{np}$ is obtained from $\eta_{pn}$ by interchanging the neutron
and proton properties. \\
The ``thermal'' processes are taken into account via fit formulae. For the 
energy emission from the {\em pair process} we use the prescription of 
Itoh et al. (1996).
%\cite{itoh96}.
 The number emission rate is obtained by deviding by the mean energy per neutrino pair (Cooperstein et al. 1986)
%\cite{cooperstein86}
\begin{equation} 
    \langle E_{\nu_i \bar{\nu}_i} \rangle_{pair}= 
    T \left( \frac{F_4(\eta_e)}{F_3(\eta_e)} 
    + \frac{F_4(-\eta_e)}{F_3(-\eta_e)} \right).
\end{equation}
For the {\em plasmon decay} we use the formulae of Haft et al. (1994)
%\cite{haft94}
with 
\begin{equation} 
    \langle E_{\nu_i \bar{\nu}_i} \rangle_{\gamma}= 
    T \left( 2 + \frac{\gamma^2}{1+\gamma} \right),
\end{equation}
where $\gamma= \gamma_0  \sqrt{\pi^2/3 + \eta_e^2}$ and $\gamma_0= 5.565
\cdot10^{-2}$.

\subsection{Diffusive Emission Rates}
In order to evaluate the opacities along given directions we map the particle
properties density, temperature and electron fraction on an 
aequidistant, cylindrical grid with coordinates $(R,Z)$, where 
$R=\sqrt{x^2+y^2}$, see Figure \ref{nugrid}. 
The assumption of rotational symmetry around the
binary rotation axis is an excellent approximation since the main neutrino
emitting region is the hot, neutron star matter debris torus that forms around
the merged central object (see Fig. 14 in paper I). 
By evaluating the EOS at each grid point the 
matter properties (like the local composition) are known 
and we can therefore  assign a variable $\zeta_{\nu_i}$ (see eq.
(\ref{zeta})), containing compositional information, to each grid point. 
The neutrino grid does not have to be 
updated at every hydro time step. We chose to update it after a small 
fraction (1/8) of the neutron star dynamical time scale, $\tau_{dyn}= 
(G \bar{\rho})^{-1/2} \approx 2 \cdot 10^{-4}$ s, which is a tiny fraction
of the timescale on which typical disk properties change.
Once all the properties on the grid are known, the desired values at 
the SPH-particle positions are found by trilinear interpolation.
We use 400 points in radial direction and 300 points in 
positive Z-direction (symmetry with respect to the orbital plane is 
an excellent approximation for the systems under investigation).

The dominant sources of opacity are
\begin{itemize}
\item [(i)] neutrino nucleon scattering: 
   \begin{equation} \nu_i + \{n, p\} \rightarrow \nu_i + \{n, p\}
   \end{equation}
   with $\sigma_{\nu_i,nuc}= \frac{1}{4} \sigma_0 \left(\frac{E_{\nu_i}}
   {m_e c^2} \right)^2$ 
%\cite{shapiro83}
(Shapiro \& Teukolsky 1983) and
\item [(ii)] coherent neutrino nucleus scattering:
   	\begin{equation}
        \nu_i + A \rightarrow \nu_i + A \label{coh_scat_formula}
   	\end{equation}
	with $\sigma_{\nu_i,A}= \frac{1}{16} \sigma_0 
	\left(\frac{E_{\nu_i}}{m_e c^2}
 	\right)^2  A^2 (1-Z/A)^2$ 
%(\cite{shapiro83}
        (Shapiro \& Teukolsky 1983; $\sin^2 \theta_W$ has 
	been approximated by 0.25). Here $A$ and $Z$ are the nucleon and 
	proton number of the average nucleus whose properties are stored in 
        our EOS-table. Due to the $A^2$-dependence of the cross section 
        this process will dominate as soon as a substantial fraction of heavy
	nuclei is present (remember that the nucleon numbers in these 
	nuclei reach values of up to $\sim$ 400 
%\cite{shen98a}
        Shen et al. 1998).\\	
	Electron type neutrinos additionally undergo
\item [(iii)] neutrino absorption:
	\begin{eqnarray}
	\nu_e + n \rightarrow p + e^-\\
	\bar{\nu}_e + p \rightarrow n + e^+
	\end{eqnarray}
	with  $\sigma_{\nu_e,n}= \frac{1+3 \alpha^2}{4} \sigma_0 
	\left(\frac{E_{\nu}}{m_e c^2}
	 \right)^2 \langle 1-f_{e^-} \rangle$, where $\langle 1-f_{e^-} 
	\rangle \approx
	\left({\rm exp}(\eta_e - F_5(\eta_{\nu_e})/F_4(\eta_{\nu_e}))+1 \right)^{-1}$\\
	and  $\sigma_{\bar{\nu}_e,p}= \frac{1+3 \alpha^2}{4} \sigma_0 
	\left(\frac{E_{\bar{\nu}}}
	{m_e c^2} \right)^2 \langle 1-f_{e^+} \rangle$, 
         $\langle 1-f_{e^+} \rangle \approx
	\left({\rm exp}(-\eta_e - F_5(\eta_{\bar{\nu}_e})/F_4(\eta_{\bar{\nu}_e})) + 1)
	\right)^{-1}$.  
\end{itemize}

The local mean free path is given by (where for simplicity the spatial
dependence is suppressed)
\begin{equation} 
	\lambda_{\nu_i}(E)= \left(\sum_r n_r \sigma_r (E)\right)^{-1}\equiv
         (E^2 \zeta_{\nu_i})^{-1} \label{zeta},
\end{equation}
where the $n_r$ denote the target number densities, the index $r$ runs 
over the reactions given above with cross-sections $\sigma_r$ and $E$ is the
neutrino energy.
The dependence of the cross-sections on the squared neutrino energies has 
been separated out in the definition of $\zeta_{\nu_i}$. The optical depth,
$\tau$, along a specified direction is then given as 
\begin{equation} 
	\tau_{\nu_i}(E)= \int_{x1}^{x2} \frac{dx}{\lambda_{\nu_i}(E)}.
\end{equation}
The optical depths are evaluated along three directions from 
each grid point: in Z-direction ($\tau^1_{\nu_i}$), 
i.e. parallel to the rotational axis, along the outgoing diagonal 
($\tau^2_{\nu_i}$) and along the ingoing diagonal ($\tau^3_{\nu_i}$), see Fig.
\ref{nugrid}.
The finally used optical depth, ($\tau_{\nu_i}$), is the minimum of the  three,
$\tau_{\nu_i}= {\rm min} (\tau^1_{\nu_i},\tau^2_{\nu_i},\tau^3_{\nu_i}$).
The quantities that are actually stored for each grid point $j$ are
\begin{equation}
	\chi^d_{j,\nu_i}= \int_{d,j} \zeta_{\nu_i}(x) dx \label{chi},
\end{equation}
where $d$ denotes the direction and $\int_{d,j} dx$ is the integration from
grid point j along direction $d$. Note that the quantity $\chi$ is independent
of the neutrino energy and the (energy dependent) optical depth is given by
\begin{equation}
\tau_{\nu_i}(E)= E^2 {\rm min}_d (\chi_{j,\nu_i}^d) \equiv E^2 \chi_{j,\nu_i}.
\label{eq_tau_without_energy}
\end{equation}

The diffusion rate depends on the optical depth \( \tau _{\nu _{i}} \). We
base our estimates on a very simple, one-dimensional diffusion
model. Along one propagation direction we assume equal probabilities for
forward and backward scattering and impose strict flux conservation in a
stationary state situation. This leads to the following relationship between
the neutrino density \( J(E) \) and the neutrino number flux \( H(E) \),
\begin{equation}
\label{eq_diffusive_flux}
\frac{H_{\nu _{i}}(E)}{cJ_{\nu _{i}}(E)}=\frac{1}{2\tau _{\nu _{i}}(E)+1}.
\end{equation}
We can test this relationship against a complete numerical solution of
the diffusion equation in e.g. a supernova environment where all relevant
opacities are included and find agreement to about a factor of two. If the
thermodynamical conditions and the neutrino densities along the propagation
direction are set, relation
(\ref{eq_diffusive_flux}) defines a local neutrino number flux \( H_{\nu_{i}}(E) \)
which in general no longer obeys flux conservation in a stationary state
situation. Assuming that we still have a stationary state situation and that
the fluxes are locally well represented, we can use the balance of fluxes
across a infinitesimally thin layer perpendicular to the propagation direction
to obtain an 
estimate of the rate \( R_{\nu _{i}} \) of neutrinos produced in this layer.
Denoting the propagation direction with \( x \), we express the rate
in terms of the prevailing neutrino density and a diffusion time scale
\( T_{\nu _{i},x}^{dif} \) with
\begin{equation}
\label{eq_diffusion_rate}
R_{\nu _{i}}^{dif}(E)=\frac{\partial H_{\nu _{i}}(E)}{\partial x}=\frac{J_{\nu _{i}}(E)}{T_{\nu _{i}}^{dif}(E)}.
\end{equation}
The substitution of eq. (\ref{eq_diffusive_flux}) for \( H_{\nu _{i}} \)
leads to spatial derivatives of the neutrino density \( J_{\nu_{i}}(E) \) and the
optical depth \( \tau_{\nu_{i}} \). As the latter is given by the negative inverse
mean free path, \( -1/\lambda _{\nu _{i}}(E) \), eq.  (\ref{eq_diffusion_rate})
can be resolved for the diffusion time scale according to
\begin{equation}
T_{\nu _{i}}^{dif}(E)=\frac{2\tau _{\nu _{i}}(E)+1}{c}\left( \frac{\partial \ln J_{\nu _{i}}(E)}{\partial x}+\frac{2}{\left( 2\tau _{\nu _{i}}(E)+1\right) \lambda _{\nu _{i}}(E)}\right) ^{-1}.
\end{equation}
We rewrite this estimate with a distance parameter, \( \Delta x(E) \), to obtain
\begin{eqnarray}
T_{\nu _{i}}^{dif}(E) & = & \frac{\Delta x_{\nu _{i}}(E)}{c}\left( 2\tau _{\nu _{i}}(E)+1\right) ,\label{eq_diffusion_time_scale} \\
\Delta x_{\nu _{i}}(E) & = & \left( \frac{\partial \ln J_{\nu _{i}}(E)}{\partial x}+\frac{2}{\left( 2\tau _{\nu _{i}}(E)+1\right) \lambda _{\nu _{i}}(E)}\right) ^{-1}.\label{eq_diffusion_distance} 
\end{eqnarray}
The spatial derivative of the neutrino density in eq. 
(\ref{eq_diffusion_distance}) is quite inconvenient, one would prefer a diffusion time scale that does not
depend on neutrino densities. Moreover,  the derivative is likely to introduce noise
when evaluated in a three-dimensional numerical simulation. Hence, we 
neglect this term. In physical terms this means that we assume neutrino sources that keep
the neutrino density close to constant over a spatial interval where the mean free path
changes significantly. This might not always be justified and is subject to future
improvement. The expression for the distance parameter, however, greatly simplifies
to
\begin{equation}
\label{eq_diffusion_dist2}
\Delta x_{\nu _{i}}(E)=\left( \tau _{\nu _{i}}(E)+\frac{1}{2}\right) \lambda _{\nu _{i}}.
\end{equation}
Here we recall that Ruffert et al. (1996)
%\cite{ruffert97a}
found the dependence
\begin{equation}
T_{\nu _{i}}^{dif}(E) = 3\frac{\Delta x_{\nu _{i}}(E)}{c}\tau _{\nu _{i}}(E)\label{Ttau}
\end{equation}
by calibration with a numerical neutrino transport scheme.
If we go back and use  \( \tau _{\nu _{i}}\sim 1 \) for the 
``last interaction region'' to simplify eq. (\ref{eq_diffusive_flux}) 
further by the approximation
\[
\frac{H_{\nu _{i}}(E)}{cJ_{\nu _{i}}(E)}=\frac{1}{3\tau _{\nu _{i}}(E)},
\]
we obtain eq. (\ref{Ttau}) by the same analysis used to derive eq. (\ref{eq_diffusion_time_scale}). However, the distance parameter is then given
by
\begin{equation}
\label{eq_diffusion_dist4}
\Delta x_{\nu _{i}}(E)=\tau _{\nu _{i}}(E)\lambda _{\nu _{i}}(E). 
\end{equation}
In our scheme  \( \Delta x \) defines the effective width of a layer drained by the
diffusive flux, i.e. provides the conversion between a net
emitted neutrino flux (number/s/cm\textasciicircum{}2)
and a production rate (number/s/cm\textasciicircum{}3).
We choose eqs. (\ref{Ttau}) and (\ref{eq_diffusion_dist4}) for our numerical
simulations because the linear dependence in \( \tau_{\nu_{i}} \) allows the
extraction of the energy dependence as in eq. (\ref{eq_tau_without_energy}).
Approximating the neutrino distribution function
in the high-density regime with a thermal equilibrium distribution we
apply the diffusion time scale and obtain the diffusion rates
\begin{equation}
	\langle R^{dif}_{\nu_i} \rangle = \int_0^\infty 
        \frac{\tilde{n}_{\nu_i}(E)}{T^{dif}_{\nu_i}(E)} dE =
	\frac{4 \pi c g_{\nu_i}}{(hc)^3} \frac{\zeta_{\nu_i}}{3 \chi^2_{\nu_i}} 
        T F_0(\eta_{\nu_i}) \label{Rdiff}
\end{equation}
\begin{equation}
	\langle Q^{dif}_{\nu_i} \rangle = \int_0^\infty 
        \frac{E \tilde{n}_{\nu_i}(E)}{T^{dif}_{\nu_i}(E)} dE =
	\frac{4 \pi c g_{\nu_i}}{(hc)^3} \frac{\zeta_{\nu_i}}{3 \chi^2_{\nu_i}} 
        T^2 F_1(\eta_{\nu_i}) \label{Qdiff}
\end{equation}
with
\begin{equation}
	\langle E^{dif}_{\nu_i} \rangle = 
        \frac{\langle Q^{dif}_{\nu_i} \rangle}{\langle R^{dif}_{\nu_i} \rangle}
	= T \frac{F_1(\eta_{\nu_i})}{F_0(\eta_{\nu_i})}.
\end{equation}
Here $\tilde{n}_{\nu_i}(E)$ is related to the number density 
by $n_{\nu_i}= \int_0^\infty \tilde{n}_{\nu_i}(E) dE$.
The statistical weights $g_{\nu_i}$ are 1 for $\nu_e$ and $\bar{\nu}_e$
and 4 for $\nu_x$. After the second equals sign in eqs. (\ref{Rdiff}) and 
(\ref{Qdiff}) we have inserted the explicit estimate (\ref{Ttau}) for 
the diffusion time scale and (\ref{eq_diffusion_dist4}) for the distance
parameter. 
Note that this leakage prescription is  {\em not} based on the use of 
mean neutrino energies, eq. (\ref{Eeff}) is exclusively used for informative 
purposes. Our scheme accounts for the energy dependence of the 
neutrino opacities by integrating over the neutrino distribution.

\end{appendix}

%%%%%%%%%%%%%%%%%%%%%%%%%%%%%%%%%%%%%%%%%%%%%%%%%%%%%%%%%%%%%%%%%%%%%%%%%%%

\end{document}
